# Supplementary material for: Auditable Versioned Data Storage Outsourcing
Source: arXiv:1507.08838 source file (2015-07-31)
Supplement: Supplementary file 1 [file f_appendix.tex]

\appendix

\section{Appendix Section}\label{app:app1}

The details of pseudo-codes
